# Supplementary material for: Projection-based significance test for longitudinally collected functional data under a crossover design
Source: arXiv:2205.08577 source file (2026-10-01)
Supplement: Supplementary file 1 [file supplement_labels.tex]

% Section, equation, figure, table and assumption numbers of the
% Supplementary Material, which the manuscript refers to.
\makeatletter
\newlabel{sec: modelformulation}{{S1}{1}{Truncated polynomial basis formula for the projected model}{}{}}
\newlabel{sec: orthogonalbasis}{{S2}{2}{Selection of the orthogonal basis}{}{}}
\newlabel{sec: discussionofassump}{{S3}{2}{Discussion of assumptions}{}{}}
\newlabel{assump: chap3mibounded}{{1}{2}{Discussion of assumptions}{}{}}
\newlabel{assump: chap3epsiloncontinuous}{{2}{2}{Discussion of assumptions}{}{}}
\newlabel{assump: chap3normality}{{3}{2}{Discussion of assumptions}{}{}}
\newlabel{assump: chap3mineigenvalue}{{4}{2}{Discussion of assumptions}{}{}}
\newlabel{sec: additionalresults}{{S4}{3}{Additional results related to PROLIFIC}{}{}}
\newlabel{theorm: chap3trtwcarrynull}{{1}{3}{Additional results related to PROLIFIC}{}{}}
\newlabel{eqn: tau_alt}{{S.1}{3}{Additional results related to PROLIFIC}{}{}}
\newlabel{eqn: chap3asymptnullqpGFtrtwcarry}{{S.2}{3}{Additional results related to PROLIFIC}{}{}}
\newlabel{theorm: chap3trtwocarrynull}{{2}{4}{Additional results related to PROLIFIC}{}{}}
\newlabel{eqn: chap3asymptnullqpGFtrtwocarry}{{S.3}{4}{Additional results related to PROLIFIC}{}{}}
\newlabel{sec: modelestimation}{{S5}{4}{Details of estimation of FACM}{}{}}
\newlabel{sec: additionalsimresults}{{S6}{4}{Additional results relevant to the simulation study}{}{}}
\newlabel{tab: size_zc}{{T1}{5}{Empirical size of \textbf {\em Ad-ZC} based on 5000 simulations}{}{}}
\newlabel{sec: additionaldataresults}{{S7}{5}{Additional figures relevant to the meloxicam study}{}{}}
\newlabel{sec: proofs}{{S8}{5}{Proof of theorems and corollaries}{}{}}
\newlabel{fig: rawandrollact}{{F1}{6}{Daily raw activity profiles for a randomly selected cat (cat number $62$) over the days $4,8,10,12$, and $16$ in all the four periods}{}{}}
\newlabel{eqn: chap3GVG}{{S.4}{6}{Proof of theorems and corollaries}{}{}}
\newlabel{fig: logcumactid1-2}{{F2}{7}{Cumulative average of the log activity profiles from $5$AM to $10$PM for two randomly selected cats (cat number $10$ and $60$) over the days $4,8,10,12$, and $16$ in all the four periods. No activities were recorded for the cat number $10$ in the last period}{}{}}
\newlabel{fig: logcumactid3-4}{{F3}{8}{Cumulative average of the log activity profiles from $5$AM to $10$PM for two randomly selected cats (cat number $36$ and $39$) over the days $4,8,10,12$, and $16$ in all the four periods}{}{}}
\newlabel{fig: freqmipandboxplots}{{F4}{9}{(a) Frequency distribution of the number of PA profiles ($m_{ip}$) observed for each of the four periods. (b) Boxplot of the baseline age (in years) and weight (in lbs) of the cats}{}{}}
\newlabel{fig: chap3allbaselinecov}{{F5}{10}{(a) Estimated mean $\widehat {\mu }(\cdot ,Age)$ at six equidistant quantiles of the distribution of $Age$ in the data, (b) Estimated effect of weight, $\widehat {\beta }_1(s)$ (c) Estimated effect of weekend, $\widehat {\beta }_2(s)$ (d) Estimated effect of DJD score, $\widehat {\beta }_3(s)$. The numbers in the y-axis are multiplied by $100$}{}{}}
\newlabel{eqn: chap3relationWdelta}{{S.5}{11}{Proof of theorems and corollaries}{}{}}
\newlabel{eqn: chap3relationdeltadelta*}{{S.6}{11}{Proof of theorems and corollaries}{}{}}
\newlabel{eqn: chap3RSS0exp}{{S.7}{11}{Proof of theorems and corollaries}{}{}}
\newlabel{eqn: chap3RSS1exp1}{{S.8}{11}{Proof of theorems and corollaries}{}{}}
\newlabel{eqn: chap3Vinvexp}{{S.9}{12}{Proof of theorems and corollaries}{}{}}
\newlabel{eqn: chap3RSS1exp2}{{S.10}{12}{Proof of theorems and corollaries}{}{}}
\newlabel{eqn: chap3RSS0expindelta}{{S.11}{12}{Proof of theorems and corollaries}{}{}}
\newlabel{eqn: chap3RSS1expindelta}{{S.12}{12}{Proof of theorems and corollaries}{}{}}
\newlabel{eqn: chap3R0-R1Expr}{{S.15}{13}{Proof of theorems and corollaries}{}{}}
\newlabel{eqn: chap3R1Expr}{{S.16}{13}{Proof of theorems and corollaries}{}{}}
\makeatother
